# Supplementary material for: Draw and Tell: Teaching Text-to-Image Diffusion Models to Describe What They Draw
Source: arXiv:2611.38889 source file (2026-11-28)
Supplement: Supplementary file 1 [file supp_main.tex]

% Draw and Tell -- CVPR 2027 submission, supplementary material (separate document).
% Build (main and supplementary cross-reference each other through xr):
%   pdflatex main; pdflatex supp; bibtex main; bibtex supp; pdflatex main; pdflatex supp; pdflatex main; pdflatex supp
% or simply:  ./build.sh
% Figures: fig/src/build.sh regenerates the TikZ/pgfplots figures in fig/; the image grids are LaTeX (fig/v3, fig/v4)
% and take their look from qualstyle.tex.
% Works two ways. Compiled on its own it is the separate document below. With \input{supp} after the bibliography of
% main.tex (Overleaf) it continues that document: same numbering and references, no second preamble.
\makeatletter
\ifx\documentclass\@notprerr
  \makeatother
  \maketitlesupplementary
  \appendix
  % \setcounter{page}{1}% submitted separately: page numbers start again
  \makeatletter\renewcommand\thesection{\ifnum\c@section>26 A\@Alph{\numexpr\c@section-26\relax}\else\@Alph\c@section\fi}\makeatother
  \setcounter{dbltopnumber}{3}\renewcommand{\dbltopfraction}{0.95}\renewcommand{\dblfloatpagefraction}{0.4}
  \input{supp_body}
  \expandafter\endinput
\fi
\makeatother
\documentclass[10pt,twocolumn,letterpaper]{article}
% \documentclass[10pt,onecolumn,letterpaper]{article}


%%%%%%%%% PAPER TYPE
\usepackage[review]{cvpr}        % REVIEW (line numbers)
% \usepackage{cvpr}              % CAMERA-READY
% \usepackage[pagenumbers]{cvpr} % arXiv version

% cvpr.sty already loads amsmath, amssymb, booktabs, graphicx, natbib, times, xcolor, xspace.
\usepackage{microtype}
\usepackage{multirow}
\usepackage{tabularx}

\usepackage{xr-hyper}            % labels of the main paper (main.aux) resolve here
\input{xrcref}                  % keep cleveref records clean when importing
\externaldocument[][nocite]{main}
\definecolor{cvprblue}{rgb}{0.21,0.49,0.74}
\usepackage[pagebackref,breaklinks,colorlinks,allcolors=cvprblue]{hyperref}
\usepackage[capitalize]{cleveref}
\crefname{appendix}{Appendix}{Appendices}\Crefname{appendix}{Appendix}{Appendices}   % sections of the supplementary

%%%%%%%%% MACROS
\newcommand{\methodlong}{Draw-and-Tell\xspace}
\newcommand{\method}{Draw\&Tell\xspace}
\newcommand{\sg}{\mathrm{sg}}
\newcommand{\Limg}{\mathcal L_{\mathrm{img}}}
\newcommand{\Ldesc}{\mathcal L_{\mathrm{desc}}}
\newcommand{\Ltxt}{\mathcal L_{\mathrm{txt}}}
\usepackage[normalem]{ulem}
\newcounter{chg}
\AtBeginDocument{\let\origcref\cref \let\origCref\Cref \let\origcite\cite}
\newcommand{\ulsafe}{%
  \renewcommand{\cref}[1]{\mbox{\origcref{##1}}}%
  \renewcommand{\Cref}[1]{\mbox{\origCref{##1}}}%
  \renewcommand{\cite}[1]{\mbox{\origcite{##1}}}}
\newcommand{\old}[1]{\stepcounter{chg}{\color{red}\textsuperscript{\thechg}\ulsafe\sout{#1}}}
\newcommand{\new}[1]{\stepcounter{chg}{\color{blue}\textsuperscript{\thechg}[#1]}}
\newcommand{\wrong}[1]{#1}                     % marks a decoded detail that contradicts the image; printed plainly

%%%%%%%%% PAPER ID
\def\paperID{*****}
\def\confName{CVPR}
\def\confYear{2027}

\title{Draw and Tell: Teaching Text-to-Image Diffusion Models\\to Describe What They Draw}

\author{Anonymous \confName~submission\\
{\tt\small Paper ID \paperID}}


\input{qualstyle}   % look of the qualitative image grids (shared with the main paper)
% float spacing; small floats are [H] (in place), wide ones go to the next page top or a float page
\setlength{\textfloatsep}{8pt plus 2pt minus 2pt}
\setlength{\floatsep}{6pt plus 2pt minus 2pt}
\setlength{\dbltextfloatsep}{8pt plus 2pt minus 2pt}
\setlength{\dblfloatsep}{6pt plus 2pt minus 2pt}
\setlength{\abovecaptionskip}{4pt}
\setcounter{dbltopnumber}{3}\renewcommand{\dbltopfraction}{0.95}\renewcommand{\dblfloatpagefraction}{0.4}
\begin{document}
\maketitlesupplementary
\appendix
\makeatletter   % sections A..Z, then AA, AB, ... (more than 26 sections)
\renewcommand\thesection{\ifnum\c@section>26 A\@Alph{\numexpr\c@section-26\relax}\else\@Alph\c@section\fi}
\makeatother

\input{supp_body}

{\small\bibliographystyle{ieeenat_fullname}\bibliography{main}}
\end{document}
